# Supplementary material for: Causally Aligned Curriculum Learning
Source: arXiv:2503.16799 source file (2025-03-21)
Supplement: Supplementary file 1 [file new_appendix.tex]

\appendix
% \section{Colored Sokoban Game}
% \label{sec:colorbox}
% This section contains the detailed setup of our Colored Sokoban game.
% \todo{colorbox details}

\section{Requirements for analyzing reward interventions}
\label{sec:no sigma y}

Unfortunately, we don't have any graphical conditions for optimal zero-shot transfer with $\sigma_Y$ edit operators as we see in Fig.~\ref{fig:sigma y mab neg}. Without changing the graphical structures, it's possible that the optimal policy in a generated source task is suboptimal in the target task. Clearly, one needs extra quantitative knowledge, which is not available under our input assumptions, to decide if a particular $\sigma_Y`$ is optimal zero-shot policy transferable.

\begin{figure}[H]
    \centering
    \includegraphics[width=\textwidth]{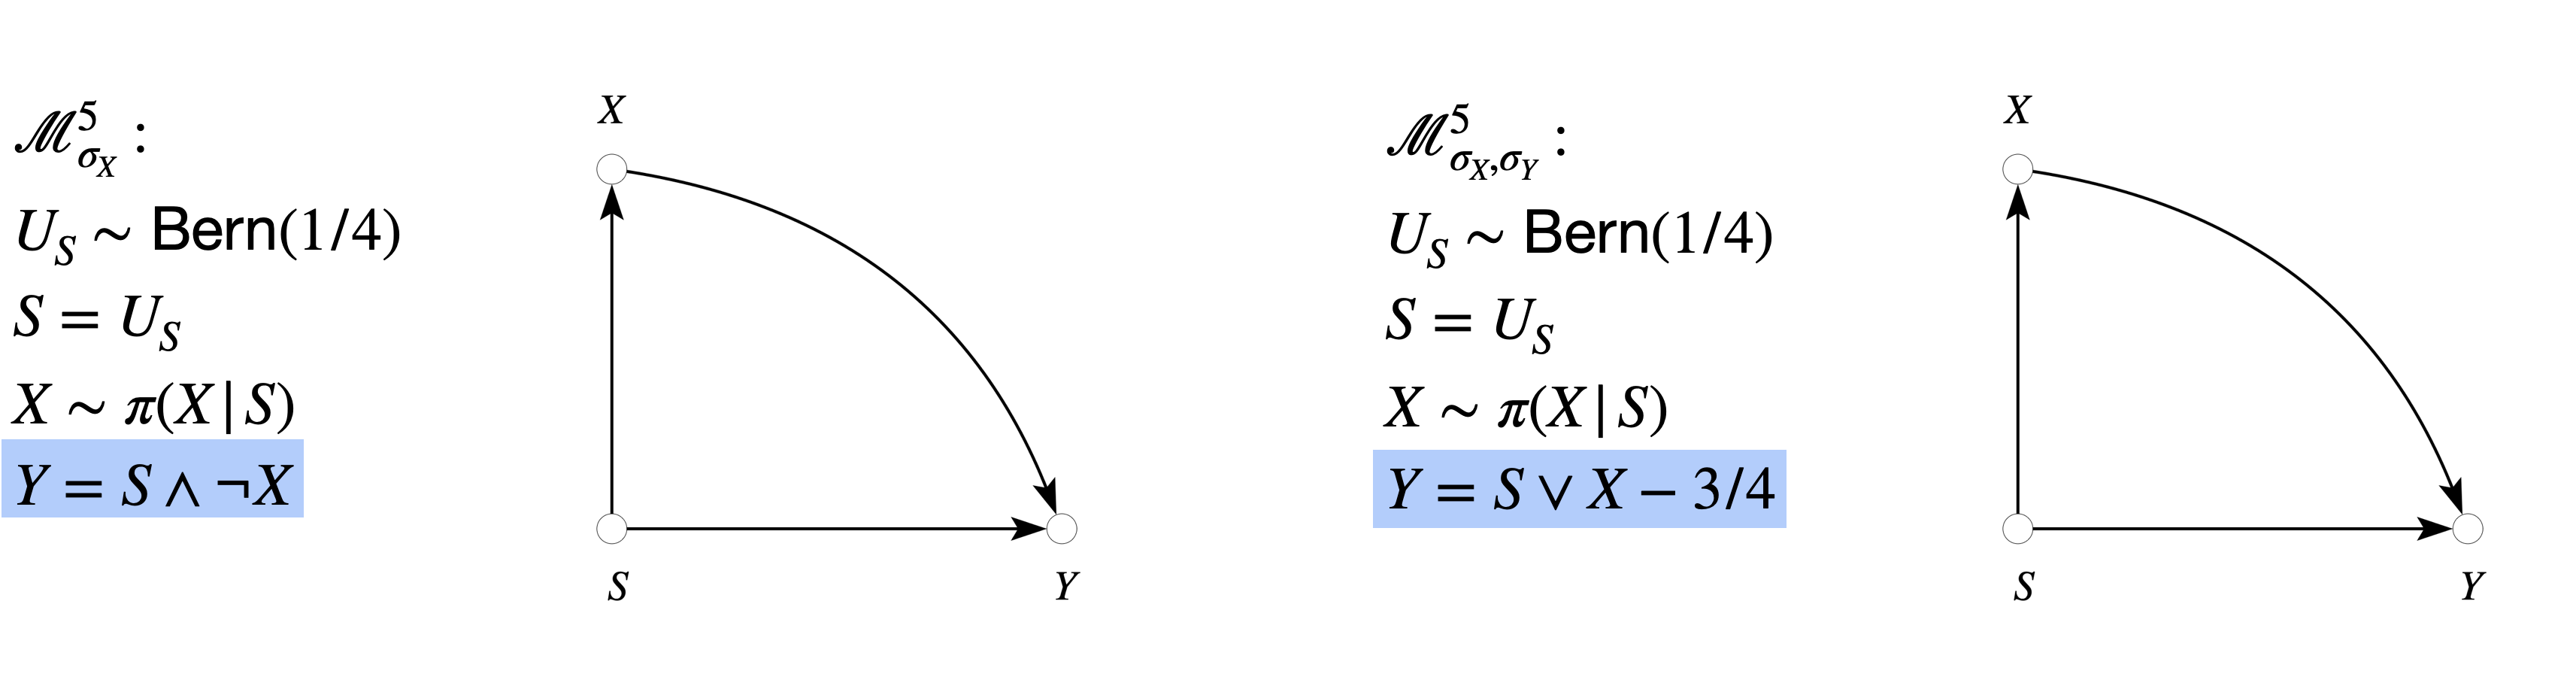}
    \caption{An example of sub-optimal zero-shot policy transfer under $\sigma$ edit applied to reward variable in single-time-step target tasks. Even the causal diagram structure stays the same under the edit, the optimal policy is different in the target task environment $\mathcal{M}^5$ and the source task environment $\mathcal{M}^5_{\sigma_Y}$. In $\mathcal{M}^5$, $\pi^*(X=1|S=1)=0$ while in $\mathcal{M}^5_{\sigma_Y}, \pi^*(X+1|S=1)=1$.}
    \label{fig:sigma y mab neg}
\end{figure}

\section{Relationship between Identifiability and Edit Admissibility}
\label{sec:relation id and admit}

\begin{example}[Identifiability and Edit Admissibility]
\label{exp:id and admissible}
\todo{add detailed derivations to these two}

	Consider a target task defined as follows, with its causal diagram shown in~\Cref{fig:criteria exp}. This target task is a two-stage sequential decision problem where action $X_1$ takes covariates $\*S_1 = \{M\}$ and action $X_2$ takes covariates $\*S_2 = \{W,Z,S\}$. The covariates' values are determined by, $M = U_M\oplus N,\ N = U_{NY_2} ,\ S = U_{SY_2}$, $Z = U_Z \oplus S$ and $W = N \oplus U_W \oplus X_1$,
    % \begin{align}
    %     W &= \begin{cases}
    %          N\oplus U_W, \text{if } X_1=1\\
    %          \neg N \oplus U_W, \text{otherwise}
    %          \end{cases}
    % \end{align}
    where the binary unobserved confounders follows distribution $P(U_M=1) = P(U_W=1) = P(U_Z=1) = P(U_{SY_2}=1) = P(U_{NY_2}=1) = 1/10$. The reward signal is defined as, $Y_1 = \neg(N \oplus X_1), Y_2 = (X_2 \oplus U_{NY_2}) \wedge U_{SY_2} \wedge Z$.
    We define source task $T^{(1)} = \tuple{\1M^{(1)},\Pi, \1R, \*V_I^{(1)}}$, where $\*V_I^{(1)} = \{M\}, M \gets 1$.
    % the effect of the decision rule $\pi_2$ on reward distribution $P^{(2)}(Y_2;\pi_2)$ is identifiable given the observational distribution of $P^{(2)}(S, W, Z, Y_2, X_2)$,
    % \begin{align}
    % 	P^{(2)}(y_2;\pi_2) = \sum_{w, z, s, x_2} P^{(2)}(y_2|z, s, x_2)\pi_2(x_2|w, z, s)P^{(2)}(w, z, s).
    % \end{align}
    The effect of this edit on the conditional reward distribution w.r.t $X_1$ is identifiable given the policy interventional distribution of $P(\*V;\pi)$,
    \begin{align}
    P^{(1)}(Y_1, Y_2\big|m,x_1;\pi)
    % \nonumber\\
    % &
    % = \sum_{n}P(Y_1\big|n, x_1; \pi)P^{(1)}(Y_2\big|n, x_1;\pi)P^{(1)}(n\big|m)\\
    % &
    = \sum_{n}P(Y_1\big|n,x_1; \pi)P(Y_2\big| n, x_1;\pi)\frac{P^{(1)}(m\big|n)P(n)}{\sum_{n'}P^{(1)}(m\big|n')P(n')}.
    \end{align} 
    So does the conditional reward distribution w.r.t $X_2$,
    \begin{align}
        P^{(1)}(Y_2\big|w,z,s,x_2;\pi) 
        % &= \sum_{n} P^{(1)}(Y_2\big|n,w,z,s,x_2;\pi)P^{(1)}(n|w;\pi) \\
        = \sum_{n} P(Y_2\big|n,z,s,x_2;\pi)\frac{\sum_{m, x_1}P(w|n,x_1;\pi)\pi(x_1\big|m)P^{(1)}(m\big|n)P(n)}{\sum_{n',x_1, m}P(w|n',x_1;\pi)\pi(x_1\big|m)P^{(1)}(m\big|n')P(n')}.
    \end{align}
    But the optimal policy learned in this source task is not optimal in the target task. The optimal target task policy is $\pi^*(X_1=M|M) = 1, \pi^*(X_2=1|S, W, Z)=1$ while the optimal source task policy is $\pi^{(1)}(X_1=\neg M|M=1) = 1, \pi^{(1)}(X_2=\neg W|S, W, Z)=1$.
%\footnote{See~\cref{sec:id derivation} for detailed identification derivations.} 
    If we define another source task $T^{(2)} = \tuple{\1M^{2},\Pi,\1R,\*V_I^{2}}$, where $\*V_I^{(2)} = \{Z\}, Z \gets 0$, clearly, we have $P^{(2)}(Y_2|W,Z,S,X_2;\pi) = P(Y_2|W,Z,S,X_2;\pi)$ since this source task satisfies our criteria, $(Y_2 \independent Z | W,S,X_2)$ in $\1G^{(2)}_{\underline{Z}}$.
    $\hfill\blacksquare$
\end{example}
\begin{figure}[t]
\centering
\hfill%
\begin{subfigure}{0.4\linewidth}\centering%(a)
  \begin{tikzpicture}
        \def\outerr{3}
        \def\innerr{2.7}
        
        \node[vertex] at (-22.50, 2.70) (W) {W};
        \node[vertex] at (-21.30, 2.70) (Z) {Z};
        \node[vertex] at (-20.10, 2.70) (S) {S};
        \node[vertex] at (-22.50, 0.90) (X2) {X\textsubscript{2}};
        \node[vertex] at (-21.30, 0.00) (Y2) {Y\textsubscript{2}};
        \node[vertex] at (-25.00, 2.70) (M) {M};
        \node[vertex] at (-23.80, 2.70) (N) {N};
        \node[vertex] at (-25.00, 0.90) (X1) {X\textsubscript{1}};
        \node[vertex] at (-23.80, 0.00) (Y1) {Y\textsubscript{1}};
        
        \draw[dir] (Z) edge [bend left=0] (X2);
        \draw[dir] (W) edge [bend left=0] (X2);
        \draw[dir] (Z) edge [bend left=0] (Y2);
        \draw[dir] (X2) edge [bend left=0] (Y2);
        \draw[dir] (S) edge [bend left=2] (X2);
        \draw[dir] (S) edge [bend left=0] (Z);
        % \draw[dir] (W) edge [bend left=0] (Z);
        % \draw[bidir] (W) edge [bend left=48] (Z);
        \draw[bidir] (S) edge [bend left=28] (Y2);
        \draw[dir] (X1) edge [bend left=0] (Y1);
        \draw[dir] (X1) edge [bend left=0] (W);
        % \draw[bidir] (M) edge [bend left=48] (N);
        \draw[dir] (N) edge [bend left=0] (W);
        % \draw[bidir] (N) edge [bend left=35] (S);
        \draw[dir] (N) edge [bend left=0] (Y1);
        \draw[dir] (M) edge [bend left=0] (X1);
        \draw[bidir] (N) edge [bend left=-33] (Y2);
        \draw[dir] (N) edge [bend left=0] (M);

	  \begin{pgfonlayer}{back}
		  \draw[fill=betterblue!25, draw = betterblue!45] \convexpath{M, X1}{\outerr mm};
		  \draw[fill=betterblue!25, draw = betterblue!45] \convexpath{W, Z, S, X2}{\outerr mm};
		  \node[circle,fill=betterblue!65,draw=none,minimum size=2*\innerr mm] at (X1) {};
		  \node[circle,fill=betterblue!65,draw=none,minimum size=2*\innerr mm] at (X2) {};
		  \node[circle,fill=betterred!65,draw=none,minimum size=2*\innerr mm] at (Y1) {};
		  \node[circle,fill=betterred!65,draw=none,minimum size=2*\innerr mm] at (Y2) {};
	  \end{pgfonlayer}
  \end{tikzpicture}
\caption{$\G$}
\label{fig:target2}
\end{subfigure}\hfill
\begin{subfigure}{0.5\linewidth}\centering%(a)
  \begin{tikzpicture}
        \def\outerr{3}
        \def\innerr{2.7}
        
        \node[vertex] at (-22.50, 2.70) (W) {W};
        \node[vertex] at (-21.30, 2.70) (Z) {Z};
        \node[vertex] at (-20.10, 2.70) (S) {S};
        \node[vertex] at (-22.50, 0.90) (X2) {X\textsubscript{2}};
        \node[vertex] at (-21.30, 0.00) (Y2) {Y\textsubscript{2}};
        \node[vertex] at (-25.00, 2.70) (M) {M};
        \node[vertex] at (-23.80, 2.70) (N) {N};
        \node[vertex] at (-25.00, 0.90) (X1) {X\textsubscript{1}};
        \node[vertex] at (-23.80, 0.00) (Y1) {Y\textsubscript{1}};

        \node[regime, betterblue, label={[shift={(-0.05,-0.05)}]\scriptsize $\tau$\textsuperscript{(1)}}] (m) at (-25.75, 2.70) {};
        \node[regime, betterblue, label={[shift={(0.35,-0.25)}]\scriptsize $\tau$\textsuperscript{(2)}}] (z) at (-21.30, 3.45) {};

	    \draw[dir, betterblue] (m) to (M);
        \draw[dir, betterblue] (z) to (Z);
        \draw[dir] (Z) edge [bend left=0] (X2);
        \draw[dir] (W) edge [bend left=0] (X2);
        \draw[dir] (Z) edge [bend left=0] (Y2);
        \draw[dir] (X2) edge [bend left=0] (Y2);
        \draw[dir] (S) edge [bend left=2] (X2);
        \draw[dir] (S) edge [bend left=0] (Z);
        % \draw[dir] (W) edge [bend left=0] (Z);
        % \draw[bidir] (W) edge [bend left=48] (Z);
        \draw[bidir] (S) edge [bend left=28] (Y2);
        \draw[dir] (X1) edge [bend left=0] (Y1);
        \draw[dir] (X1) edge [bend left=0] (W);
        % \draw[bidir] (M) edge [bend left=48] (N);
        \draw[dir] (N) edge [bend left=0] (W);
        % \draw[bidir] (N) edge [bend left=35] (S);
        \draw[dir] (N) edge [bend left=0] (Y1);
        \draw[dir] (M) edge [bend left=0] (X1);
        \draw[bidir] (N) edge [bend left=-33] (Y2);
        \draw[dir] (N) edge [bend left=0] (M);

	  \begin{pgfonlayer}{back}
		  \draw[fill=betterblue!25, draw = betterblue!45] \convexpath{M, X1}{\outerr mm};
		  \draw[fill=betterblue!25, draw = betterblue!45] \convexpath{W, Z, S, X2}{\outerr mm};
		  \node[circle,fill=betterblue!65,draw=none,minimum size=2*\innerr mm] at (X1) {};
		  \node[circle,fill=betterblue!65,draw=none,minimum size=2*\innerr mm] at (X2) {};
		  \node[circle,fill=betterred!65,draw=none,minimum size=2*\innerr mm] at (Y1) {};
		  \node[circle,fill=betterred!65,draw=none,minimum size=2*\innerr mm] at (Y2) {};
	  \end{pgfonlayer}
  \end{tikzpicture}
  \caption{$\G^{(1)}$ and $\G^{(2)}$}
  \label{fig:source2}
  \end{subfigure}\hfill\null
  \caption{
  An example on admissibility is not identifiability. \subref{fig:target2}) causal diagram for the target task $T$; and (\subref{fig:source2}) comparing domain discrepancies between the target task $T$ and source tasks $T^{(1)}$ and $T^{(2)}$.
  }
  \label{fig:criteria exp}
\end{figure}

\section{Correctness of Algorithms}
\label{sec:correctness of search alg}
asdfasdf

\section{Proof for theorems}

In this section, we provide proof sketches for all the theorems proposed in the previous sections.
\begin{proof}[\textbf{Optimal Curriculum Learning (\Cref{thm:curriculum_learning})}]
Since we have an policy that is optimal in every source task,
\begin{align}
    \pi^*(\1C) = \argmax_{\pi \in \Pi} \InvE{\1R(\*Y)}{\pi}{\1M^{(j)}}, \forall  T^{(j)} \in \1C. 
\end{align}
And for each action, we have $\D(\*S_i) \subseteq \bigcup_{T^{(j)} \in \1C[X_i]} \D(\*S_i; \pi^{(j)})$. These two together imply that $\pi^*(\1C)$ acts optimally $X_i \in \*X$ in every situation $\D(\*S_i)$. Thus, $\pi^*(\1C)$ is optimal in the target task by definition.
\end{proof}

\begin{proof}[\textbf{Equivalent Criteria for Admissible States}]
In \cref{def:admissible states}, the graphical criterion is 
\begin{align}
    (\*V_I^{(j)} \independent \*Y_{X} \big|X, \*S_{X}\setminus \*V_I^{(j)}) \text{ in } \mathcal{G}'_{\underline{\*V_I^{(j)}\cap 
    \*S_{X}}\overline{\*V_I^{(j)}(X)}} \label{eq:criteria}
\end{align}
where 
$\*Y_{X} \subseteq \*Y \cap \De(X)$,
and
$\overline{\*V_I^{(j)}(X)}=\*V_I^{(j)}\setminus \An(X)$.

We would like to show that it is equivalent to having each edited state variable $V\in\*V_I^{(j)}$ satisfying the following,
\begin{align}
    (V \independent \*Y_{X} \big|X, \*S_{X}\setminus \{V\}) \text{ in } \mathcal{G}'_{\underline{{\{V\}}\cap 
    \*S_{X}}\overline{\{V\}(X)}}\label{eq:equivalent}
\end{align}
where 
$\*Y_{X} \subseteq \*Y \cap \De(X)$, 
and $\overline{\{V\}(X)}=\{V\}\setminus \An(X)$.

Firstly, we show that if \Cref{eq:criteria} is violated, \Cref{eq:equivalent} must also be violated. We observe that when \Cref{eq:equivalent} is violated, there exists a variable $V\in\*V^{(j)}$ such that $(V \notindependent \*Y_{X} \big|X, \*S_{X}\setminus \*V_I^{(j)}) \text{ in } \mathcal{G}'_{\underline{\*V_I^{(j)}\cap 
    \*S_{X}}\overline{\*V_I^{(j)}(X)}}$. Then for the set of edit variables $\*V^{(j)}_I \cap \*S_X\setminus \{V\}$, their outgoing edges are all cut out and having them in the conditioning set will only opens up collider paths (if there are any) but not blocking paths. So, we have $(V \notindependent \*Y_{X} \big|X, \*S_{X}\setminus \{V\}) \text{ in } \mathcal{G}'_{\underline{\*V_I^{(j)}\cap 
    \*S_{X}}\overline{\*V_I^{(j)}(X)}}$. Clearly, \Cref{eq:equivalent} uses the same independence check but only in a graph with more edges added to this one. Thus, if \Cref{eq:criteria} is violated, the same independence check cannot hold since adding edges won't create independence~\citep{pearl2009causality}.

Secondly, we show that if a single edited state variable, $V\in \*V^{(j)}$ violates the equivalent criteria \Cref{eq:equivalent}, \Cref{eq:criteria} must also be violated. There are three possibilities,

\begin{enumerate}[label=\roman*), left=0pt, topsep=0pt, parsep=0pt]
	\item If $V\in \*S_X$ and $(V \notindependent \*Y_{X} \big|X, \*S_{X}\setminus \{V\}) \text{ in } \1G'_{\underline{V}}$, this indicates that there is a d-connected path $p$ of the following form: $V\leftarrow \cdots \cdot Y$. Assume \Cref{eq:criteria} holds. There exists a node $Z$ s.t. $Z\in \*V_I^{(j)}$ and $p$ is blocked in \Cref{eq:criteria}due to either $Z\in \*S_X\cap \*V_I^{(j)}$ being a descendant of a collider on $p$ or an edge associated with $Z$ being cut out. 
		If $Z\in \*S_X$ is a descendant of a collider $V'$ on $p$ and $p$ is open due to having $Z$ in conditioning set of \Cref{eq:equivalent}, the graph looks like follows,
		\begin{figure}[H]
		\centering
		\includegraphics[width=.8\textwidth]{pics3/23.png}
		\end{figure}
		There exists a path $p' = Z \leftarrow \cdots \leftarrow V' \leftarrow \cdots \cdots \rightarrow Y$. We see that $X$ cannot observe any other variables on the causal path from $V'$ to $Z$ because that opens the collider path. The path between $V' \leftarrow \cdots V'' \cdots \rightarrow Y$ also cannot be blocked under \Cref{eq:criteria}. If it is blocked, there exists a variable $V''\in \*V_I^{(j)}$ such that an edge is cut out. $V''\notin \*S_X$ as that will block $p$ under \Cref{eq:equivalent}. So $V'' \notin \An(X)$ and an incoming edge to $V''$ is cut out. This also means that on the LHS of $V''$, there should be another collider s.t. $V''\notin \An(X)$ but this contradicts with the setting that $p$ is open under \Cref{eq:equivalent}. 
	 	Then, we have $Z\notin \*S_X$ and it's on the path $p$ s.t. an edge associated with $Z$ is cut out under \Cref{eq:criteria} so $p$ is blocked. Then we have $Z \notin \An(X)$ and edges associated with $Z$ must be in the form of $\leftarrow Z \leftarrow$ or $\rightarrow Z \rightarrow$. Since we also have $Z\in \*V_I^{(j)}$, it must be independent from $Y$, so the RHS path from $Z$ to $Y$ cannot be open under \Cref{eq:criteria}, which means the path takes the form of $V \leftarrow \cdots \leftarrow Z \leftarrow \cdots Y$ (we are in a finite SCM so we can assume there won't be other edited variables on RHS of $Z$ s.t. $p$ is blocked). We also have the constraint that $Z \notin \*S_X$. There must exist a converging point like $V \leftarrow \cdots \rightarrow Z' \leftarrow Z \leftarrow \cdots Y$. The problem is that $p$ is blocked only because $Z$'s edges being cut out, under which $\De(Z')$ must be observed to keep the LHS path of $Z$ open. But again, this makes $Z\in \An(X)$ contradicting to our conditions.
	\item If $V\notin \An(X)$, $(V \notindependent \*Y_{X} \big|X, \*S_{X}) \text{ in } \mathcal{G}_{\overline{V}}$, and we assume \Cref{eq:criteria} holds, as analyzed in previous case, there must exist a node $Z$ on a d-connected path $p$, s.t. $Z\in \*V_I^{(j)}$, $p$ is blocked in \Cref{eq:criteria} due to an edge associated with $Z$ being cut out. As the same reason in previous case, $Z \in \*V_I^{(j)}$ and $Z$ itself satisfies \Cref{eq:criteria}. Thus, $p$ must be in the form of $V\rightarrow \cdots \leftarrow Z \leftarrow \cdots Y$. Then, there exists a collider node $Z'$ between $V$ and $Z$ s.t. $\De(Z')$ is observed. This reduces to the same scenario as in previous case. So, this also cannot happen.	
	\item If $V\in \An(X)\setminus\*S_X$, $(V \notindependent \*Y_{X} \big|X, \*S_{X}) \text{ in } \mathcal{G}$ and we assume \Cref{eq:criteria} holds, as analyzed in previous case, there must exist a node $Z$ on a d-connected path $p$, s.t. $Z\in \*V_I^{(j)}$, $p$ is blocked in \Cref{eq:criteria} due to an edge associated with $Z$ being cut out. Like the previous case, path $p$ must be in the form of $V \cdots \leftarrow Z \leftarrow \cdots Y$ and $Z \notin \An(X)$. Then there exists a collider $Z'$ between $V$ and $Z$ being open, and $\De(Z')$ is observed, which again contradicts to the condition that $Z \notin \An(X)$.
\end{enumerate}
Thus, \Cref{eq:equivalent} is equivalent to \Cref{eq:criteria}.
\end{proof}

\begin{proof}[\textbf{Sufficiency of the new criterion (\Cref{thm:aligned source task})}]
Since we the relevance graph is acyclic, each action can be optimized solely w.r.t to its reward signals $\*Y_X$ and find its optimal decision rule.
Our goal is to show that if the set of edited state variables, $\*V_I^{(j)}$, satisfies our criterion, the optimal decision rule for an action $X\in\*X^{(j)}$ stays invariant,
\begin{align}
    \argmax_{\pi}\InvE{\1R(\*Y_{X})}{\pi}{\1M} = \argmax_{\pi}\InvE{\1R(\*Y_{X})}{\pi}{\1M^{(j)}}.\label{eq:central equation}
\end{align}

This is equivalent to having, for any $\*s_X \in \*S_X$,
\begin{align}
	  &\argmax_{\pi(\cdot|\*s_X)}\sum_{\*y, x}\1R(\*y_X)P(\*y_X|\*s_X, x)\pi(x|\*s_X)\nonumber\\
	= &\argmax_{\pi(\cdot|\*s_X)}\sum_{\*y, x}\1R(\*y_X)P^{(j)}(\*y_X|\*s_X, x)\pi(x|\*s_X).
\label{eq:invariant eq}
\end{align}

By \Cref{thm:equivalent admissible}, we only need to show that \Cref{eq:invariant eq} holds under \Cref{eq:equivalent}.
%, the sufficiency of \Cref{eq:equivalent} will be proved. 
Specifically, we would like to show that $P(\*y_X|\*s_X, x) = P^{(j)}(\*y_X|\*s_X, x)$ if each variable edited, $V \in \*V_I^{(j)}$, satisfies \Cref{eq:equivalent}. There are three possibilities,
\begin{enumerate}[label=\roman*), left=0pt, topsep=0pt, parsep=0pt]
    \item If $V \in \*S_{X}$, by \Cref{eq:equivalent}, we have $(V\independent\*Y_{X}\big|\*S_{X}\setminus \{V\}, X)$ in $\1G_{\underline{V}}$, which is exactly Rule 2 of the do-calculus. Thus, editing on such $V$ won't change this conditional reward distribution;
    \item If $V \notin \An(X)$, we can cut the incoming edges of such $V$, and again \Cref{eq:equivalent} gives us exactly Rule 3 of the do-calculus. Thus, editing on such $V$ won't change this conditional reward distribution;
    \item If $V \in \An(X) \setminus\*S_{X}$, similar to the previous case,  \Cref{eq:equivalent} gives us Rule 3 of the do-calculus. The only difference is that no edges can be cut out this time. Thus, editing on such $V$ still won't change this conditional reward distribution.
\end{enumerate}

We have shown that all the regime indexes can be removed from the inside of the $\argmax$ operator and thus have successfully proved~\Cref{eq:invariant eq} under \Cref{eq:equivalent}, which validates our criteria's sufficiency. 
\end{proof}

\begin{proof}[\textbf{Necessity of the new criterion (\Cref{thm:aligned source task})}]

To show our criterion is necessary, it amounts to show that given a causal diagram, $\1G$, whenever the criterion is violated by editing in a non-admissible set of variables, $\*V_I^{(j)}$, there always exists a pair of target task $T$ and a source task $T^{(j)}$ that are compatible with $\1G$ but have different optimal policies for an action $X\in \*X^{(j)}$. 
By \Cref{thm:equivalent admissible}, when the criterion is violated, there exists at least a variable $V\in\*V_I^{(j)}$ and an action $X \in \*X^{(j)}$ such that $(V\notindependent \*Y_{X} \big| \*S_X\setminus\*V_I^{(j)}, X)$ in graph $\1G_{\underline{\*V_I^{(j)}\cap\*S_X}\overline{\*V_I^{(j)}(X)}}$. This indicates the existence of an open path from this variable $V$ to a reward signal, $Y \in \*Y_X$. 

Firstly, we establish that when the criteria is violated, there always exists an open path $p$ from $V$ to $Y$ such that there are no other action nodes on the path. To prove, we assume that there exists an action $X_2$ on path $p$ and $V$ violates the criteria w.r.t $X_1 \in \*X^{(j)}$. Since $p$ is open under $X_1, \*S_{X_1}\setminus \{V\}$, any action variable on this path satisfies $X_2 \prec X_1$. Based on the LHS edge direction of $X_2$, there are two possibilities.
\begin{enumerate}[label=\roman*), left=0pt, topsep=0pt, parsep=0pt]
	\item If the LHS of $X_2$ is an outgoing edge, the graph looks like follows.
		\begin{figure}[H]
		\centering
		\includegraphics[width=.8\textwidth]{pics4/1.png}
		\end{figure}
	In this case, there can be no colliders between $V, X_2$ since $p$ is open under $X_1, \*S_{X_1}\setminus \{V\}$ and observing the descendants of these colliders creates loops. So, the path from $X_2 \rightarrow \cdots \rightarrow V$ must be causal. Again, to avoid loops, $V\notin \An{X_1}$. By our criteria, we can cut all incoming edges of $X_1$, which means that $X_1$ cannot violate the criteria contradicting to the condition that $V$ violates the criteria. Thus, this case is impossible to happen.
	\item If the LHS of $X_2$ is an incoming edge, the graph looks like follows.
		\begin{figure}[H]
		\centering
		\includegraphics[width=.8\textwidth]{pics4/2.png}
		\end{figure}
	$X_2$ must observe some variable, say $V_1$, on the causal path from $X_1$ to $Y$ to avoid cyclic $\1G_r$. There is also an open path $p'$ connecting $X_2$'s LHS parent to $Y$ since it cannot be an irrelevant observation. Now, this creates a new path $V \cdots V_2 \cdots p' \cdots Y$ from $V$ to $Y$. If there are no other actions on $p'$, the only way that is blocked under \Cref{eq:equivalent} is that $p'$ contains $\*S_{X_1}$ \todo{or has colliders observed by X2}. This is impossible because $p'$ is open under $\*S_{X_2}\setminus V_2$ and this will create a cyclic $\1G_r$ between $X_1$ and $X_2$. So, if there are no other actions nor $\*S_{X_1}$ on this new path $p'$, it is an open path, which satisfies our argument. But if there exists an action $X_3$ on $p'$, we can also show that this is actually impossible. Assume there exists such an $X_3$ and the graph looks like,
		\begin{figure}[H]
		\centering
		\includegraphics[width=.8\textwidth]{pics3/9.png}
		\end{figure}
		$X_3$ must observe some variable on both path of $X_2 \cdots Y_2$ and $X_1 \cdots Y$ to avoid cyclic $\1G_r$. Now, if LHS of $X_3$ is an incoming edge, this again loops back to our analysis on $X_2$ \todo{which request another $X_4 \prec X_3$ to avoid irrelevant observations???. But this cannot go infinitely as we are in a finite SCM.} Thus, there must exist a base case where the LHS of $X_3$ is an outgoing edge. But this still cannot happen because to avoid loop in the path $X_3 \rightarrow V_3 \cdots V_2 \rightarrow X_2 \longrightarrow X_3$, there must exist a collider between $V_2$ and $V_3$. But $p'$ should also be open under $\*S_{X_2}\setminus V_2$ which means that $X_2$ is one of the descendants of this collider. This again creates a loop. Thus, there will always be an open path $p$ without any actions between $V$ and $Y$. And we will use this path for all the following counter example constructions.
\end{enumerate}

Secondly, we start with the easier scenario where there are no causal paths from $X$ to $Y$ such that there are other actions on the path. If $V$ violates the criterion, based on its type, we can construct counter examples as follows. Note that we assume $\De(\*Y) = \emptyset$ since this is a common condition in the influence diagram literature\citep{PGMbook} and reinforcement learning literature\citep{rlbook}, and rewards are also usually a human-designed signal external to the environment dynamics.
\begin{enumerate}[label=\roman*), left=0pt, topsep=0pt, parsep=0pt]
    \item If $V \in \*S_{X}$ and $(V \notindependent \*Y_{X} \big|\*X_{\preceq X}, \*S_{X}\setminus \{V\}) \text{ in } \1G'_{\underline{V}}$, there exists an open path $p$ without any other action nodes from $V$ to $Y$. The graph looks like follows,
		\begin{figure}[H]
		\centering
		\includegraphics[width=.8\textwidth]{pics3/10.png}
		\end{figure}
		By this edge direction, there must exist a common cause node $V_1$ on this path (could be a confounder). And we assume $V_1$ is the rightmost common cause on this $p$ path. We can now construct the misaligned source task, target task pair as follows. In the target task, let all other rewards $\*Y\setminus Y$ yield zero but only $Y = \neg (A\oplus B)$, which means that $X$ is only optimized towards this $Y$. All non-collider variables other than $X, Y$ copy its parent's value on these two paths between $X, Y$. Variables without endogenous parents act like a fair coin. For colliders, it takes bit-parity of all its inputs on these two paths. In the source task, we let $V = \neg \pa_V$ instead of copying its parent's value as in the target. 
		If $V_1 \rightarrow \cdots \rightarrow V$ is causal, the policy is misaligned because,
		\begin{align}
		\pi^*(X = V \big | V) = 1, \pi'(X = \neg V \big | V) = 1 
		\end{align}
		where $\pi^*$ is the optimal target task policy and $\pi'$ is the optimal source task policy.
		If $V_1 \rightarrow \cdots \rightarrow V$ is not causal, there are colliders between $V_1$ and $V$. The graph looks like the following,
		\begin{figure}[H]
		\centering
		\includegraphics[width=.8\textwidth]{pics3/11.png}
		\end{figure}
		Assume $V_2$ is such a collider on path $p$. There won't be other action $X'$ between $V_2, X$ because that results in $X'\prec X$ and leads to a causal path from $X$ to $Y$ with other actions, $X \rightarrow \cdots \rightarrow X' \rightarrow Y$, which violates our setting. Then we have $X\in\De(V_2)$. If there are no other colliders between $V_2$ and $V$, the optimal policy for the target and the source are (for simplicity, we write $X$ as conditioning directly on $V_2$),
		\begin{align}
			\pi^*(X=V\oplus V_2 \big | V, V_2) = 1, \pi'(X=\neg V\oplus V_2 \big | V, V_2) = 1
		\end{align}
		If there are more colliders between $V$ and $V_2$, say $V_3, V_4, ...$, we can still have the same set up. The source task will still be misaligned because,
		\begin{align}
			&\pi^*(X=V\oplus V_2 \oplus V_3 \oplus \cdots \big | V, V_2, V_3, ...) = 1\\
			&\pi'(X=\neg V\oplus V_2 \oplus V_3 \oplus \cdots \big | V, V_2, V_3, ...) = 1
		\end{align}
		
    \item If $V \notin \An(X)$ and it satisfies $V \notindependent Y \big | \*S_X, \*X_{X \preceq X})$ in $\1G'_{\overline{V}}$, the graph looks like,
		\begin{figure}[H]
		\centering
		\includegraphics[width=.8\textwidth]{pics3/12.png}
		\end{figure}
		The path from $V$ to $Y$ must be causal because any colliders between $V, Y$ result in either causal path between $X, Y$ with other actions or $V$ being ancestors of $X$. Following the same set up in previous case, but now we let all variables without endogenous variables, i.e. $V$, act like a biased coin with $P(V=1) = 1/4$ in the target while in the source it's edited to be $P(V=1) = 3/4$. Clearly, the optimal target policy and source policy is not aligned as,
		\begin{align}
			\pi^*(X=0) = 1, \pi'(X=1)=1.
		\end{align}

    \item If $V \in \An(X)\setminus \*S_{X}$ and it satisfies $(V \notindependent Y \big|\*X_{\preceq X}, \*S_{X}) \text{ in } \1G'$, the graph looks like,
		\begin{figure}[H]
		\centering
		\includegraphics[width=.8\textwidth]{pics3/13.png}
		\end{figure}
		Since we let every intermediate nodes copy its parent value, case (b) can be reduced to the construction in (i). We only need to discuss (a) then. We follow the same set up as in (i). The only differences are that in target we let $P(V=1) = 1/4$ and $V_1 = V\vee U_{V_1}, P(U_{V_1} = 1) = 99/100$ and in source we let $P(V=1) = 3/4$.
		If the path from $V$ to $Y$ is causal, clearly, the optimal policy is not aligned,
		\begin{align}
			\pi^*(X=0|V_1=1) = 1, \pi'(X=1|V_1=1)=1.
		\end{align}
%		Note that $X$ won't observe any variables on the $V,Y$ causal path directly because that will render the $V_1$ an irrelevant observation so this construction is valid.
		If the path from $V$ to $Y$ is not causal, there exists colliders between $V$ and $Y$, say $V_2, V_3, ...$, and the graph looks like this,
		\begin{figure}[H]
		\centering
		\includegraphics[width=.8\textwidth]{pics3/14.png}
		\end{figure}	
		We can still use the same set up and the optimal policies are not aligned since,
		\begin{align}
			&\pi^*(X = V_1\oplus V_2 \oplus \cdots | V_1=1, \*S_X) = 1,\\
			&\pi'(X = \neg V_1 \oplus V_2 \oplus \cdots | V_1=1, \*S_X)=1.
		\end{align}
%		For the same reason, $X$ won't observe any variables on the $V,Y$ causal path after the rightmost collider on this $V, Y$ path so this construction is valid.
\end{enumerate}

Thirdly, we will construct counter examples for the last possible scenario when there exists causal paths with other action nodes on it. We denote the variable being edited as $V_1$ and we want to show that as $V_1$ violates the criterion, the optimal policy of action $X_1$ is not invariant.
\begin{enumerate}[label=\roman*), left=0pt, topsep=0pt, parsep=0pt]
    \item If $V_1 \in \*S_{X_1}$, we construct examples based on different number of action nodes on the $X\rightarrow \cdots \rightarrow Y$ path. 
		\begin{enumerate}[left=0pt, topsep=0pt, parsep=0pt]
			\item If there is only one action node, the graph looks like follows,
				\begin{figure}[H]
				\centering
				\includegraphics[width=.8\textwidth]{pics3/15.png}
				\end{figure}
				WLOG, we can assume $X_2$ directly observes $X_1$. To avoid cyclic $\1G_r$, $X_2$ must observe a variable on the open path $p$ from $V$ to $Y$. From the edge type, there exists at least one common cause node, say $V_2$ on $p$. Assume $V_2$ is the rightmost common cause to $Y$. If there are more common cause node on $p$, there will also be colliders. Since $p$ is open under our criteria, those colliders must have actions $X_{\preceq X_1}$ as descendants. As our set up in previous cases, values are copied from each node's parent. Thus $X_2$ can always recover the true $V_2$ value by receiving all colliders values and take bit parity of them. So, for simplicity, we can assume there is only one common cause on $p$ and $X_2$ observes $V_2$ directly. 
				There is another path $p'$ from $X_1$ to $Y$. This is because $X_1$ shouldn't be an irrelevant observation to $X_2$. So, there must be an open path from $X_1$ to $Y$ under observations $\*S_{X_2}\setminus X_1$. On this $p'$ path, the downside edge with $X_1$ must be an outgoing edge since $\1G_r$ is acyclic. If this path is causal, the graph looks like follows,
					\begin{figure}[H]
					\centering
					\includegraphics[width=.8\textwidth]{pics3/16.png}
					\end{figure}
					$V_3$ cannot be an irrelevant observation to $X_3$ so there will be another open path linking $V_3$ to $Y$ under $\*S_{X_3}\setminus V_3$, which is exactly the same situation as we are analyzing for $X_2$. Since we are in a finite SCM, there exists base cases for this situation. So, $p'$ is either a $X_3$ free causal path or a path with colliders, which we will cover next. If  $p'$ is a causal path without other actions, we can continue to use the same construction as we do when there exists causal paths without actions previously.
					Then, for the case when there are colliders in $p'$, they must have $X_2$ as descendants because this path should be open when $\*S_{X_2} \setminus X_1$ is given. The graph looks like follows,
					\begin{figure}[H]
					\centering
					\includegraphics[width=.8\textwidth]{pics3/17.png}
					\end{figure}
					There cannot be other action nodes before the last common cause node (e.g, no actions can exist between $V_4, V_5$) because $p'$ is open and $X_2$ is a descendant of all such colliders, this will result in cyclic $\1G_r$.
					There could only be other actions after the last common cause node on $p'$, which is also on a causal path towards $Y$ and the graph looks like follows,
					\begin{figure}[H]
					\centering
					\includegraphics[width=.8\textwidth]{pics3/18.png}
					\end{figure}
					In this case, there will also be an open path from $V_4$ to $Y$ such that $V_4$ is not an irrelevant observation for $X_3$. But again this new path and $X_3$ fit into the same analysis as we do for $X_2$. Since there won't be infinitely many new action nodes, the base case is that there is no action nodes on such path like $p'$. Now we are only left to construct misaligned tasks for a graph like follows,
					\begin{figure}[H]
					\centering
					\includegraphics[width=.8\textwidth]{pics3/17.png}
					\end{figure}
					WLOG, let $V_5$ be the rightmost collider on $p'$, $V_3$ be the leftmost collider on $p'$ and $V_4$ be the second leftmost collider. (There could be more colliders between $V_3, Y$. Assume there are only three for now.) If not defined particularly, we let every non-collider covariate copy its parent values on the path in this graph and every non-collider covariate without endogenous parents in this graph act as a fair coin. For colliders, they always output the bit parity of all the inputs from nodes in this graph. We let $Y$ take a 2-bit input and,
					\begin{align}
						Y = \begin{cases}
						\neg (B\ //\ 2)\oplus C,\ \text{if } A = 1\\
						\neg (B\ \mathrm{mod}\ 2)\oplus C,\ \text{if } A = 0\\
						\end{cases}
					\end{align}
					The core construction comes to the common cause between $V_3, V_4$. Say it's $V_{41}$. We let it output a 2 bit value where each bit act as an independent fair coin. However, $V_3$ only reveals part of the information to its descendants based on $X_1$'s input,
					\begin{align}
						V_3 = \begin{cases}
						\neg (V_{41}\ //\ 2),\ \text{if } X_1 = 1\\
						\neg (V_{42}\ \mathrm{mod}\ 2),\ \text{if } X_1 = 0\\
						\end{cases}
					\end{align}
					For $V_4$, let its RHS parent be $V_{42}$. $V_4$ yields a 2 bits value composed of bit parities with each bit from $V_{41}$, $V_4 = \left(V_{42}\oplus (V_{41} \ //\ 2), V_{42}\oplus (V_{41} \ \mathrm{mod}\ 2)\right)$. Thus, to act optimally w.r.t $Y$, $X_2$ must decode the last common cause node's value between $V_5, Y$ by taking bit parities of all the input value it receives from these colliders and output a 2-bits value, $X_2 = \left(V_5 \oplus V_{42} \oplus (V_{41}\ // \ 2) \oplus V_3, V_5 \oplus V_{42} \oplus (V_{41}\ \mathrm{mod} \ 2) \oplus V_3) \right)$. By the property of bit-parity, $X_2$'s output is actually $X_2 = \left( C \oplus (V_{41}\ // \ 2) \oplus V_3, C \oplus (V_{41}\ \mathrm{mod} \ 2) \oplus V_3)\right)$. In the target task where $V_1$ copies its parent's value, the optimal policy for $X_1$ is also copying values so $V_3$ will reveal the correct bit required by $Y$. For example, if $V_2 = 0$, $A=0$ and $Y$ will check the last bit of $X_2$. Since $V_3$ also reveals $V_{41} \ \mathrm{mod}\ 2$, the last bit of $X_2$ will be exactly $C$ and get the optimal reward. However, if we now flip the output of $V_1$ in a source task, the optimal policy will have to flip this value back so $V_3$ can reveal the correct bit to $X_2$. Thus, this pair of tasks are misaligned. If there are more colliders between $V_3, Y$, we can still use a similar construction with only $X_2$ taking a few more values from those extra colliders. They will cancel out each other without affecting our conclusion of misaligned tasks.
			\item If there are multiple action nodes on the causal path from $X_1$ to $Y$, the graph looks like follows,
				\begin{figure}[H]
				\centering
				\includegraphics[width=.8\textwidth]{pics3/19.png}
				\end{figure}
				The same analysis and construction still applies because there still exists $p'$ such that $X_1$ is not an irrelevant observation. Even if there are other covariates between $X_1, X_2$, the $p'$ path will only change its starting point from $X_1$ to the corresponding covariate, which won't affect our construction. And the same decoding work has to be done by the rightmost action node on this $X_1, X_2, ..., X_3, Y$ causal path. All actions before that one only need to pass down any observed colliders' values to it (if there are any).
 		\end{enumerate}
    \item If $V_1 \notin \An(X_1)$, there is no way that $X_1$ can ever know what value $V_1$ is and the $p$ path from $V_1$ to $Y$ must be causal as we have analyzed previously. So, we can let $V_1$ act as a biased coin such that $P(V_1=1) = 1/100$. Then we can use the same construction as in previous case. The only difference is that in target task, the optimal policy for $X_1$ is to output $0$ all the time. In source tasks, if we let $P(V_1=1) = 99/100$, $X_1$'s optimal policy will also need to be flipped. Thus, it's still misaligned. Note that it doesn't matter whether the rightmost action on the $X_1 \rightarrow \cdots \rightarrow Y$ causal path observes values on $p$ or not since the distribution is biased it can also lean towards one $v_1$ value and be optimal.
    \item If $V_1 \in \An(X_1)\setminus \*S_{X_1}$, we can transform this case back to similar situations of the previous two cases and use their constructions. The graph now looks like follows,
		\begin{figure}[H]
		\centering
		\includegraphics[width=.8\textwidth]{pics3/20.png}
		\end{figure}
		Firstly, we establish that there will be no other actions $X'$ on the causal path between $V_1, X_1$. If there is one, $X'$, since $p$ is open under $X_1$'s observations, we have $X'\prec X_1$. To avoid cyclic relevance graph, $X'$ has to observe a variable on the causal path from $X$ to $Y$, which creates a loop. Then, if $V_1$ is not a common cause, $X_1 \leftarrow V_2 \leftarrow \cdots \leftarrow V_1 \leftarrow$, we can let every variable between $V_1, X_1$ copy parent's value on this path and reuse the same analysis when $V_1\in\*S_{X_1}$. If $V_1$ is a common cause, $X_1 \leftarrow V_2 \leftarrow \cdots \leftarrow V_1 \leftarrow$, we can let $V_2$ add a lot noise to its parent's value, e.g., $V_2 = U \vee V_1, P(U=1)=99/100$. When $V_2 = 1$, $X_1$ has no valuable information about $V$ so we can reuse the constructions in previous case. Even if $V_1$ is a common cause and path $p$ from $V_1$ to $Y$ is not causal, due to acyclic relevance graph and our copying value set up, there will always be an action observing all colliders and cancels those values out by taking bit parity as if there are no colliders on the path $p$. So the same construction still applies.
\end{enumerate}

Thus, we have shown that once our criterion is violated, there always exists a target task $T$ and a source task $T^{(j)}$ that are compatible in the causal diagram but not aligned in the optimal policy of an action $X_1 \in \*X^{(j)}$.
\end{proof}

\begin{proof}[\textbf{Unique Maximum Admissible Sets (\Cref{thm:unique maximum})}]
	Let $K = \max_{\*V_I^{(j)}} |\*V_I^{(j)}|$. If there are two maximal admissible sets $\*V_1, \*V_2$ w.r.t $\*X{(j)}$, they satisfy $|\*V_1| = |\*V_2| = K$ but $\*V_1 \neq \*V_2$. Interchangably, we can assume that there exists a state variable $V\in \*V_1$ but $V\notin \*V_2$. By \Cref{thm:equivalent admissible}, $V$ satisfies our criterion, so does every variable in $\*V_2$. Then by \Cref{thm:equivalent admissible} again, we know the set $\*V' = \*V_2 \cup \{V\}$ is admissible w.r.t $\*X^{(j)}$, which contradicts with the fact that $\*V_2$ is the maximal set since $|\*V' | = K+1$. Thus, this is impossible to happen.
\end{proof}

\begin{proof}[\textbf{Existence of $\pi^*(\1C)$ (\Cref{thm:pic existence})}]
We can argue that for a curriculum that satisfies $\D(\*S_i) \subseteq \bigcup_{T^{(j)} \in \1C[X_i]} \D(\*S_i; \pi^*(\1C))$ and \Cref{thm:pic existence}, the union of all optimal decision rules learned in those source tasks is $\pi^*(\1C)$. Firstly, for a policy to be optimal in a source task $T^{(j)}$, by \Cref{thm:pic existence}, it only needs to be optimal in actions $\*X^{(j)}$. Secondly, the optimal decision rule of an action $X$ learned in source task $T^{(j)}$ will not be overwritten after taking the union because \Cref{thm:pic existence} guarantees that the invariant action set is expanding, $\*X^{(j)} \subseteq \*X^{(j+1)}$, which implies that optimal decision rules of $X$ will be invariant whenever it is learned in a source task. Thus, $\pi^*(\1C) = \bigcup_{T^{(j)}\in\1C} \pi^{(j)}$ where $\pi^{(j)}$ is the optimal policy of source task $T^{(j)}$.
\end{proof}

\section{Experiment and Implementation Details}
\label{sec:exp details}
This section introduces the detailed setup of our experiments including environment specifications, hyper-parameters, agent structures, and testing protocols.

\section{Related Work}
\label{sec:related work}
\input{sections_tex/related_work}
